# Supplementary material for: Dynamical Mean-Field Theory Simulations with the Adaptive Sampling Configuration Interaction Method
Source: arXiv:1711.04771 source file (2019-10-03)
Supplement: Supplementary file 1 [file SuppInfo.pdf]

# Next Generation Dynamical Mean-Field Theory Simulations with the Adaptive Sampling Configuration Interaction Method - Supporting Information

Carlos Mejuto-Zaera, Norm M. Tubman\*, K. Birgitta Whaley

\*Corresponding author: ntubman@berkeley.edu

University of California, Berkeley, California 94720, United States

(Dated: April 16, 2019)

## SUPPORTING INFORMATION

Here we present bullet point flow charts for the DMFT and ASCI algorithms. "Ground state" is shortened as GS. A brief physical motivation of the impurity model is also in order: In DMFT, quantum fluctuations outside from the cluster sites is accounted for by introducing the fermionic bath site degrees of freedom. The possibility for a particle to leave the cluster, move through the rest of the lattice and finally return to the cluster is thus represented by the couplings to the single bath sites. From this interpretation it becomes clear that an infinite number of bath degrees of freedom is formally needed to recover the thermodynamic limit behavior of the system. Since exact diagonalization or configuration interaction solver force finite baths, studying the effect of this bath discretization error becomes fundamental to evaluate the validity of DMFT calculations.

TABLE I. DMFT method [1]

|                   |                                                                                                                                                                                                                                                                                                                                                                                                                                                                                                                                                                                                                                                                                                                                                                                                                                                                                                                                                                                                                                                                                                                                                                                                                                                                                                                                                                                                                                                                                                                                                                                                                                                                                                                                                                                                                                                                                                                                                                                                                                                                                                                                                       |
|-------------------|-------------------------------------------------------------------------------------------------------------------------------------------------------------------------------------------------------------------------------------------------------------------------------------------------------------------------------------------------------------------------------------------------------------------------------------------------------------------------------------------------------------------------------------------------------------------------------------------------------------------------------------------------------------------------------------------------------------------------------------------------------------------------------------------------------------------------------------------------------------------------------------------------------------------------------------------------------------------------------------------------------------------------------------------------------------------------------------------------------------------------------------------------------------------------------------------------------------------------------------------------------------------------------------------------------------------------------------------------------------------------------------------------------------------------------------------------------------------------------------------------------------------------------------------------------------------------------------------------------------------------------------------------------------------------------------------------------------------------------------------------------------------------------------------------------------------------------------------------------------------------------------------------------------------------------------------------------------------------------------------------------------------------------------------------------------------------------------------------------------------------------------------------------|
| <u>Input:</u>     | Number of cluster sites $N_c$ , Number of bath sites $N_b$ , Hamiltonian $H$ .                                                                                                                                                                                                                                                                                                                                                                                                                                                                                                                                                                                                                                                                                                                                                                                                                                                                                                                                                                                                                                                                                                                                                                                                                                                                                                                                                                                                                                                                                                                                                                                                                                                                                                                                                                                                                                                                                                                                                                                                                                                                        |
| <u>Output:</u>    | Bath parameters $E_p$ , $V_{p,\alpha}$ ( $p \in [1, N_b]$ , $\alpha \in [1, N_c]$ ).                                                                                                                                                                                                                                                                                                                                                                                                                                                                                                                                                                                                                                                                                                                                                                                                                                                                                                                                                                                                                                                                                                                                                                                                                                                                                                                                                                                                                                                                                                                                                                                                                                                                                                                                                                                                                                                                                                                                                                                                                                                                  |
| <u>Algorithm:</u> | <ol style="list-style-type: none"> <li>1. Initial guess for bath parameters. Usually this comes from a low level calculation, like Hartree-Fock.</li> <li>2. Compute GS wave function <math> GS\rangle</math> and energy <math>E_{GS}</math> of current impurity model with the impurity solver.</li> <li>3. Compute cluster Green's function <math>G_c(i\omega)</math> and self energy <math>\Sigma_c(i\omega)</math>. These are <math>(N_c \times N_c)</math> matrices defined as <math>G_{c,(\alpha,\beta)}(i\omega) = \langle GS   c_\alpha \frac{1}{i\omega + \mu - (H - E_{GS})} c_\beta^\dagger   GS \rangle + \langle GS   c_\beta^\dagger \frac{1}{i\omega + \mu + (H - E_{GS})} c_\alpha   GS \rangle</math> and <math>\Sigma_c(i\omega) = G_0^{-1}(i\omega) - G_c(i\omega)</math>, where <math>c_\alpha</math>, <math>c_\beta^\dagger</math> are the annihilation and creation operators for cluster sites <math>\alpha</math> and <math>\beta</math> respectively, <math>G_0(i\omega)</math> is the non-interacting Green's function of the impurity model and <math>\mu</math> is the chemical potential.</li> <li>4. Compute local full lattice Green's function from the cluster Green's function by Fourier transforming <math>G(i\omega, \mathbf{R}) = \frac{1}{V_{BZ}} \int_{BZ} d\mathbf{k} \exp(i\mathbf{k} \cdot \mathbf{R}) [(i\omega + \mu) - h(\mathbf{k}) - \Sigma_c(i\omega)]^{-1}</math>. Here <math>h(\mathbf{k})</math> is the Fourier transform of the non-interacting part of <math>H</math> with respect to the unit cell defined by the cluster and <math>BZ</math> stands for the Brillouin zone defined by the same unit cell. To recover the Green's function on the cluster, we set <math>\mathbf{R} = \mathbf{R}_0 \equiv \mathbf{0}</math>.</li> <li>5. Impose self-consistency <math>G_c(i\omega) = G(i\omega, \mathbf{R}_0)</math>. This means that we can express <math>G(i\omega, \mathbf{R}_0)</math> with the bath parameters.</li> <li>6. Find new bath parameters by fitting <math>G(i\omega, \mathbf{R}_0)</math>.</li> <li>7. If bath parameters converged, finish. If not, go to step 2.</li> </ol> |

[1] D. Zgid and G. K.-L. Chan, J. Chem. Phys. **134**, 094115 (2011).

[2] N. M. Tubman, J. Lee, T. Y. Takeshita, M. Head-Gordon, and K. B. Whaley, J. Chem. Phys. **145**, 044112 (2016).

[3] N. M. Tubman, C. D. Freeman, D. S. Levine, D. Hait, M. Head-Gordon, and B. Whaley, ArXiv e-prints (2018), arXiv:1807.00821 [quant-ph].

TABLE II. ASCI method [2, 3]

|                   |                                                                                                                                                                                                                                                                                                                                                                                                                                                                                                                                                                                                                                                                                                                                                               |
|-------------------|---------------------------------------------------------------------------------------------------------------------------------------------------------------------------------------------------------------------------------------------------------------------------------------------------------------------------------------------------------------------------------------------------------------------------------------------------------------------------------------------------------------------------------------------------------------------------------------------------------------------------------------------------------------------------------------------------------------------------------------------------------------|
| <u>Input:</u>     | Size $tdets$ of the target space $\{D_{tdets}\}$ , size $cdets$ of the core space $\{D_{search}\}$ , Hamiltonian $H$ , basis (usually localized orbital basis).                                                                                                                                                                                                                                                                                                                                                                                                                                                                                                                                                                                               |
| <u>Output:</u>    | Optimal target space of size $tdets$ , ground state energy $E_{GS}$ and wavefunction $ GS\rangle$ .                                                                                                                                                                                                                                                                                                                                                                                                                                                                                                                                                                                                                                                           |
| <u>Algorithm:</u> | <ol style="list-style-type: none"> <li>1. Initial guess for target space. This can be a Hartree-Fock solution plus single and double excitations.</li> <li>2. Compute GS in current target space.</li> <li>3. Find connected singles and doubles to the <math>cdets</math> most important target space states (the core space). Most important means largest coefficient in the GS wavefunction.</li> <li>4. Rank all states, target space plus the singles and doubles from the core space, according to Eq. 10.</li> <li>5. Update the target space by choosing the top <math>tdets</math> states of the ranking in step 4.</li> <li>6. Compute GS in the new target space.</li> <li>7. If GS energy is converged, finish. If not, go to step 3.</li> </ol> |

TABLE III. This work - ASCI-DMFT (Calculating the Green's function)

|                    |                                                                                                                                                                                                                                                                                                                                                                                                                                                                                                                                                                                                                                                                                                                                                                                                                                                                                                                                                                                                                                                                                                                                                                                                                                                                                                                                                                                                                                                                                                                                                                                                                                                                                                                                                                                                                                                                                                                                                                                                                                                                                                                                                                                                                                                                                                        |
|--------------------|--------------------------------------------------------------------------------------------------------------------------------------------------------------------------------------------------------------------------------------------------------------------------------------------------------------------------------------------------------------------------------------------------------------------------------------------------------------------------------------------------------------------------------------------------------------------------------------------------------------------------------------------------------------------------------------------------------------------------------------------------------------------------------------------------------------------------------------------------------------------------------------------------------------------------------------------------------------------------------------------------------------------------------------------------------------------------------------------------------------------------------------------------------------------------------------------------------------------------------------------------------------------------------------------------------------------------------------------------------------------------------------------------------------------------------------------------------------------------------------------------------------------------------------------------------------------------------------------------------------------------------------------------------------------------------------------------------------------------------------------------------------------------------------------------------------------------------------------------------------------------------------------------------------------------------------------------------------------------------------------------------------------------------------------------------------------------------------------------------------------------------------------------------------------------------------------------------------------------------------------------------------------------------------------------------|
| <u>After ASCI:</u> | <p>Find spaces for particle and hole excitations. This is needed to compute the cluster Green's function as shown in Table I. We need to find the zero states connected to each of the <math>c_\alpha^\dagger\{D_{tdets}\}</math> and <math>c_\alpha\{D_{tdets}\}</math>, where <math>\alpha</math> runs over all cluster sites. For the diagonal elements of <math>G_c(i\omega)</math>, one proceeds as:</p> <ol style="list-style-type: none"> <li>1. Act with the creation operator on the ASCI target space. The states reached this way form the core of the single particle excitation space.</li> <li>2. Find all zero states connected to the <math>m</math> leading states and add them to the target space. Zero states are single and double excitations on top of the states found in step 8. Rather than fixing a number <math>m</math>, we introduce a lower cutoff for the absolute value of the ground state coefficient. We only find zero states for states with absolute coefficients above the cutoff. Additional layers of zero are added until convergence is reached. An additional layer of zero states means to add the zero states connected to the zero states of a previous layer. For the systems studied in this work, one layer is enough along the imaginary frequency axis, while the real axis requires two layers.</li> <li>3. Proceed analogously with the annihilation operator for the single hole excitation</li> </ol> <p>For the off-diagonal element <math>(\alpha, \beta)</math> of <math>G_c(i\omega)</math>, one proceeds by computing the Green's function for <math>c_\alpha^\dagger \pm c_\beta^\dagger</math>. Additional states might need to be added if there are zero states connected to the <math>(\alpha, \alpha)</math> space that can only be reached from the <math>(\beta, \beta)</math> space and vice-versa.</p> <p>Adding these steps to the ASCI algorithm presented in Table II provides a functional impurity solver for DMFT.</p>                                                                                                                                                                                                                                                                                                   |
| <u>Example:</u>    | <p>Consider a 1 dimensional system of spinless fermions with five sites for the fermions to reside. Any state in this system of fermions can be described in second quantization as <math> n_1 n_2 n_3 n_4 n_5\rangle</math>, where <math>n_i</math> is the occupation number for site <math>i</math>. The number of particles <math>N = \sum_{i=1}^5 n_i</math> is an integer between 0 and 5. Let us assume that the target space <math>\{D_{tdets}\}</math> of the ASCI calculation has 2 fermions. A possible state would be <math> 00011\rangle \in \{D_{tdets}\}</math>. When computing the Green's function matrix element <math>(1, 1)</math>, we will act with <math>c_1^\dagger</math> on <math>\{D_{tdets}\}</math>. This will map <math> 00011\rangle \rightarrow  10011\rangle</math>. <math> 10011\rangle</math> is an element of the core single particle excitation space for the <math>(1,1)</math> element of the Green's function (In contrast, when computing the corresponding single hole excitation space, the state <math> 00011\rangle</math> would not contribute, since it is mapped to zero by the annihilation operator <math>c_1</math>). Now, to complete the single particle excitation space, we want to add zero states, i.e. <math>N+1</math> (in this case 3) particle states that are connected by the Hamiltonian to <math>c_1^\dagger\{D_{tdets}\}</math>. Those are states with <math>n_1 = 0</math>. Now, which states are connected to the core single particle excitation space depends on the nature of the Hamiltonian. For the sake of our example, we will assume that <math>H</math> only includes nearest neighbor hopping terms, connecting state <math>i</math> with states <math>i+1</math> and <math>i-1</math> (with periodic boundary conditions). Thus, from <math> 10011\rangle</math> we can only reach the zero states <math> 01011\rangle</math> and <math> 10101\rangle</math>, any other 3-fermion state with <math>n_1 = 0</math> cannot be reached from <math> 10011\rangle</math> by nearest neighbor hops. Thus, we would only add <math> 01011\rangle</math> and <math> 10101\rangle</math>. This process has then to be repeated for each state in <math>\{D_{tdets}\}</math> and for each creation and annihilation operator.</p> |
